# Supplementary material for: Multi-Agent Active Search using Realistic Depth-Aware Noise Model
Source: arXiv:2011.04825 source file (2021-03-22)
Supplement: Supplementary file 1 [file 6-supplementary.tex]

\clearpage

\rule{\columnwidth}{0.13cm}
\begin{center}
	\LARGE \bf 
	Supplementary material:\\
	Multi-Agent Active Search using \\ Realistic Depth-Aware Noise Model
\end{center}
\rule{\columnwidth}{0.04cm}

\vspace{0.3cm}
\begin{abstract}
	This document provides a short description on the submitted video demonstrations.
\end{abstract}

\section*{Video Demonstration}

%\subsection*{First Video}
Video \textbf{``1-demonstration.mp4''} provides a demonstration of how NATS performs in our Unreal environment. The first 38 seconds of the video is a short introduction on the details of the environment's appearance. The video then starts a demonstration of the algorithm. Here, the top half of the screen provides the movements of the two robots Agent 0 and Agent 1 as the explore the environment. Each agent includes a small map on the top right corner displaying the agent's location at any time. The lower half of the screen presents the details of our algorithm NATS as it updates its estimate of the detected locations as more measurements become available. 

We note here that the algorithm is not on any central planner. In fact, this animation is a demonstration of NATS algorithm on both Agent 0 and 1 as it updates the available measurements by all the agents. As a result, there is some timing delay between when the agent make an observation and when the observation updates the belief of the algorithm for the agents.

By the end of this video, we see that using NATS has helped the two agents to explore the environment almost entirely. At this point, we can see that the agents have located 5 out of 6 objects of interest. 
%We consider the person in the center of the map being successfully located. The exact location of this person is difficult to estimate due to high levels of hills and mountains around this region. 
As apparent in the video, the two agents have done a great job covering the entire map avoiding each other sensing regions. Lastly, we see that the agents were unsuccessful in locating one person in the center of the map. The location of this person is difficult to estimate due to high levels of hills and mountains around this region. NATS has reported high levels of uncertainty there which suggests that allowing more measurements can lead to locating this last person.
%his lack of success is due to object detector's low accuracy in detecting this person even in close proximity as the region is under large shadows of mountains. 
%We will next show a detailed demonstration of the NATS algorithm for the same example showing that NATS, in fact, made a nonzero estimate on presence of a person in that location.

\begin{rem}
	We would like to here again emphasize that the object detector YOLOv3 used in this experiment is using weights trained on COCO dataset and there has been 
	\emph{no training} on our UE4 environment.
	\end{rem}

\begin{rem}
	We would like to also emphasize that for simplicity the robot planning video in this supplementary is not including path planning and mapping. In other words, a real robot will not necessarily pick the straight line path from one sensing action to the next. 
\end{rem}
